# Supplementary material for: Towards Auditing Unsupervised Learning Algorithms and Human Processes For Fairness
Source: arXiv:2209.11762 source file (2022-09-20)
Supplement: Supplementary file 1 [file supplement.tex]

\begin{center}
\underline{\underline{\Large{\textbf{Supplementary Material}}}}
\end{center}

\bigskip

\noindent
\textsf{Paper title:}~{\large Testing for Clustering Unfairness:}
                      {\large A Combinatorial Optimization Approach}

\iffalse
%%%%%%%%%%%%%%%%%%%%%%%%%%%%%%%%%%%%%%%%%%%%%%%%%%%%%
\noindent
\begin{tabular}{ll}
{\large\textsf{Paper title:}} & {\large Testing for Clustering Unfairness:}\\
                              & {\large A Combinatorial Optimization Approach}\\
\end{tabular}
%%%%%%%%%%%%%%%%%%%%%%%%%%%%%%%%%%%%%%%%%%%%%%%%%%%%%
\fi

\bigskip

\section{Additional Experimental Results}

Here, we include some additional experimental results.

\begin{figure*}[h]
\begin{center}
\includegraphics[scale=0.6]{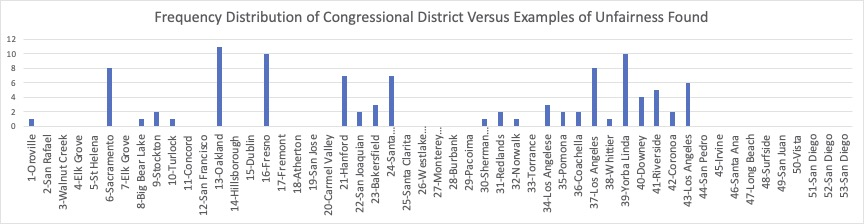}
\end{center}
\caption{Additional experimental results for Section \ref{sec:exp2}.
This figure shows the distribution of the 50 shortest explanations/examples of
unfairness across California's 53 congressional districts. The
x-axis refers to the congressional district number and the y-axis indicates
how often unfairness was found in the district.}
\label{fig:census}
\end{figure*}

\bigskip

\begin{table*}[h]
\begin{center}
\begin{tabular}{|c|}
\hline
Wed Apr 01 22:39:24 +0000 2015|Blood test for Down's syndrome hailed \\http://bbc.in/1BO3eWQ
ttp://bbc.in/1ChTANp \\ \hline
Wed Apr 08 18:05:28 +0000 2015|New approach against HIV 'promising' \\ http://bbc.in/1E6jAjt \\ \hline
Thu Apr 09 01:31:50 +0000 2015|Breast cancer risk test devised \\ http://bbc.in/1CimpJF \\ \hline
Tue Apr 07 00:04:09 +0000 2015|Why strenuous runs may not be so bad after all \\ http://bbc.in/1Ceq0Y7 \\ \hline
Mon Apr 06 07:46:44 +0000 2015|VIDEO: Health surcharge for non-EU patients \\ http://bbc.in/1C5Mlbk \\ \hline
\end{tabular}
\end{center}
\caption{Additional information on the data set used in Section \ref{sec:exp3}. 
This table shows a few examples of articles on health from the BBC health care
website. The first article would be tagged as being on handicapped,
the third about women and the fifth about poverty. 
Note that the tagging is based on an article's content and not its title.}
\label{tab:exfeeds}
\end{table*}
